# Supplementary material for: Human Multi-View Synthesis from a Single-View Model:Transferred Body and Face Representations
Source: arXiv:2412.03011 source file (2024-12-04)
Supplement: Supplementary file 1 [file X_suppl.tex]

\clearpage
\setcounter{page}{1}
\setcounter{section}{0}
\maketitlesupplementary

\section*{Overview}
\label{sec:supp_overview}
This supplementary material is organized as follows:
\begin{itemize}
\item We first introduce the additional qualitative results on THuman2.1 in Section \ref{sec:supp_mutli_qualitative_res}.
\item We then introduce the additional qualitative results from 3D gaussian splatting in Section \ref{sec:supp_gs_qualitative_res}.
\item We finally provide the additional ablation studies of the architecture of our method in Section \ref{sec:supp_abl}. 
\end{itemize}
%.
\begin{figure}
\centering
\includegraphics[width=1\linewidth]{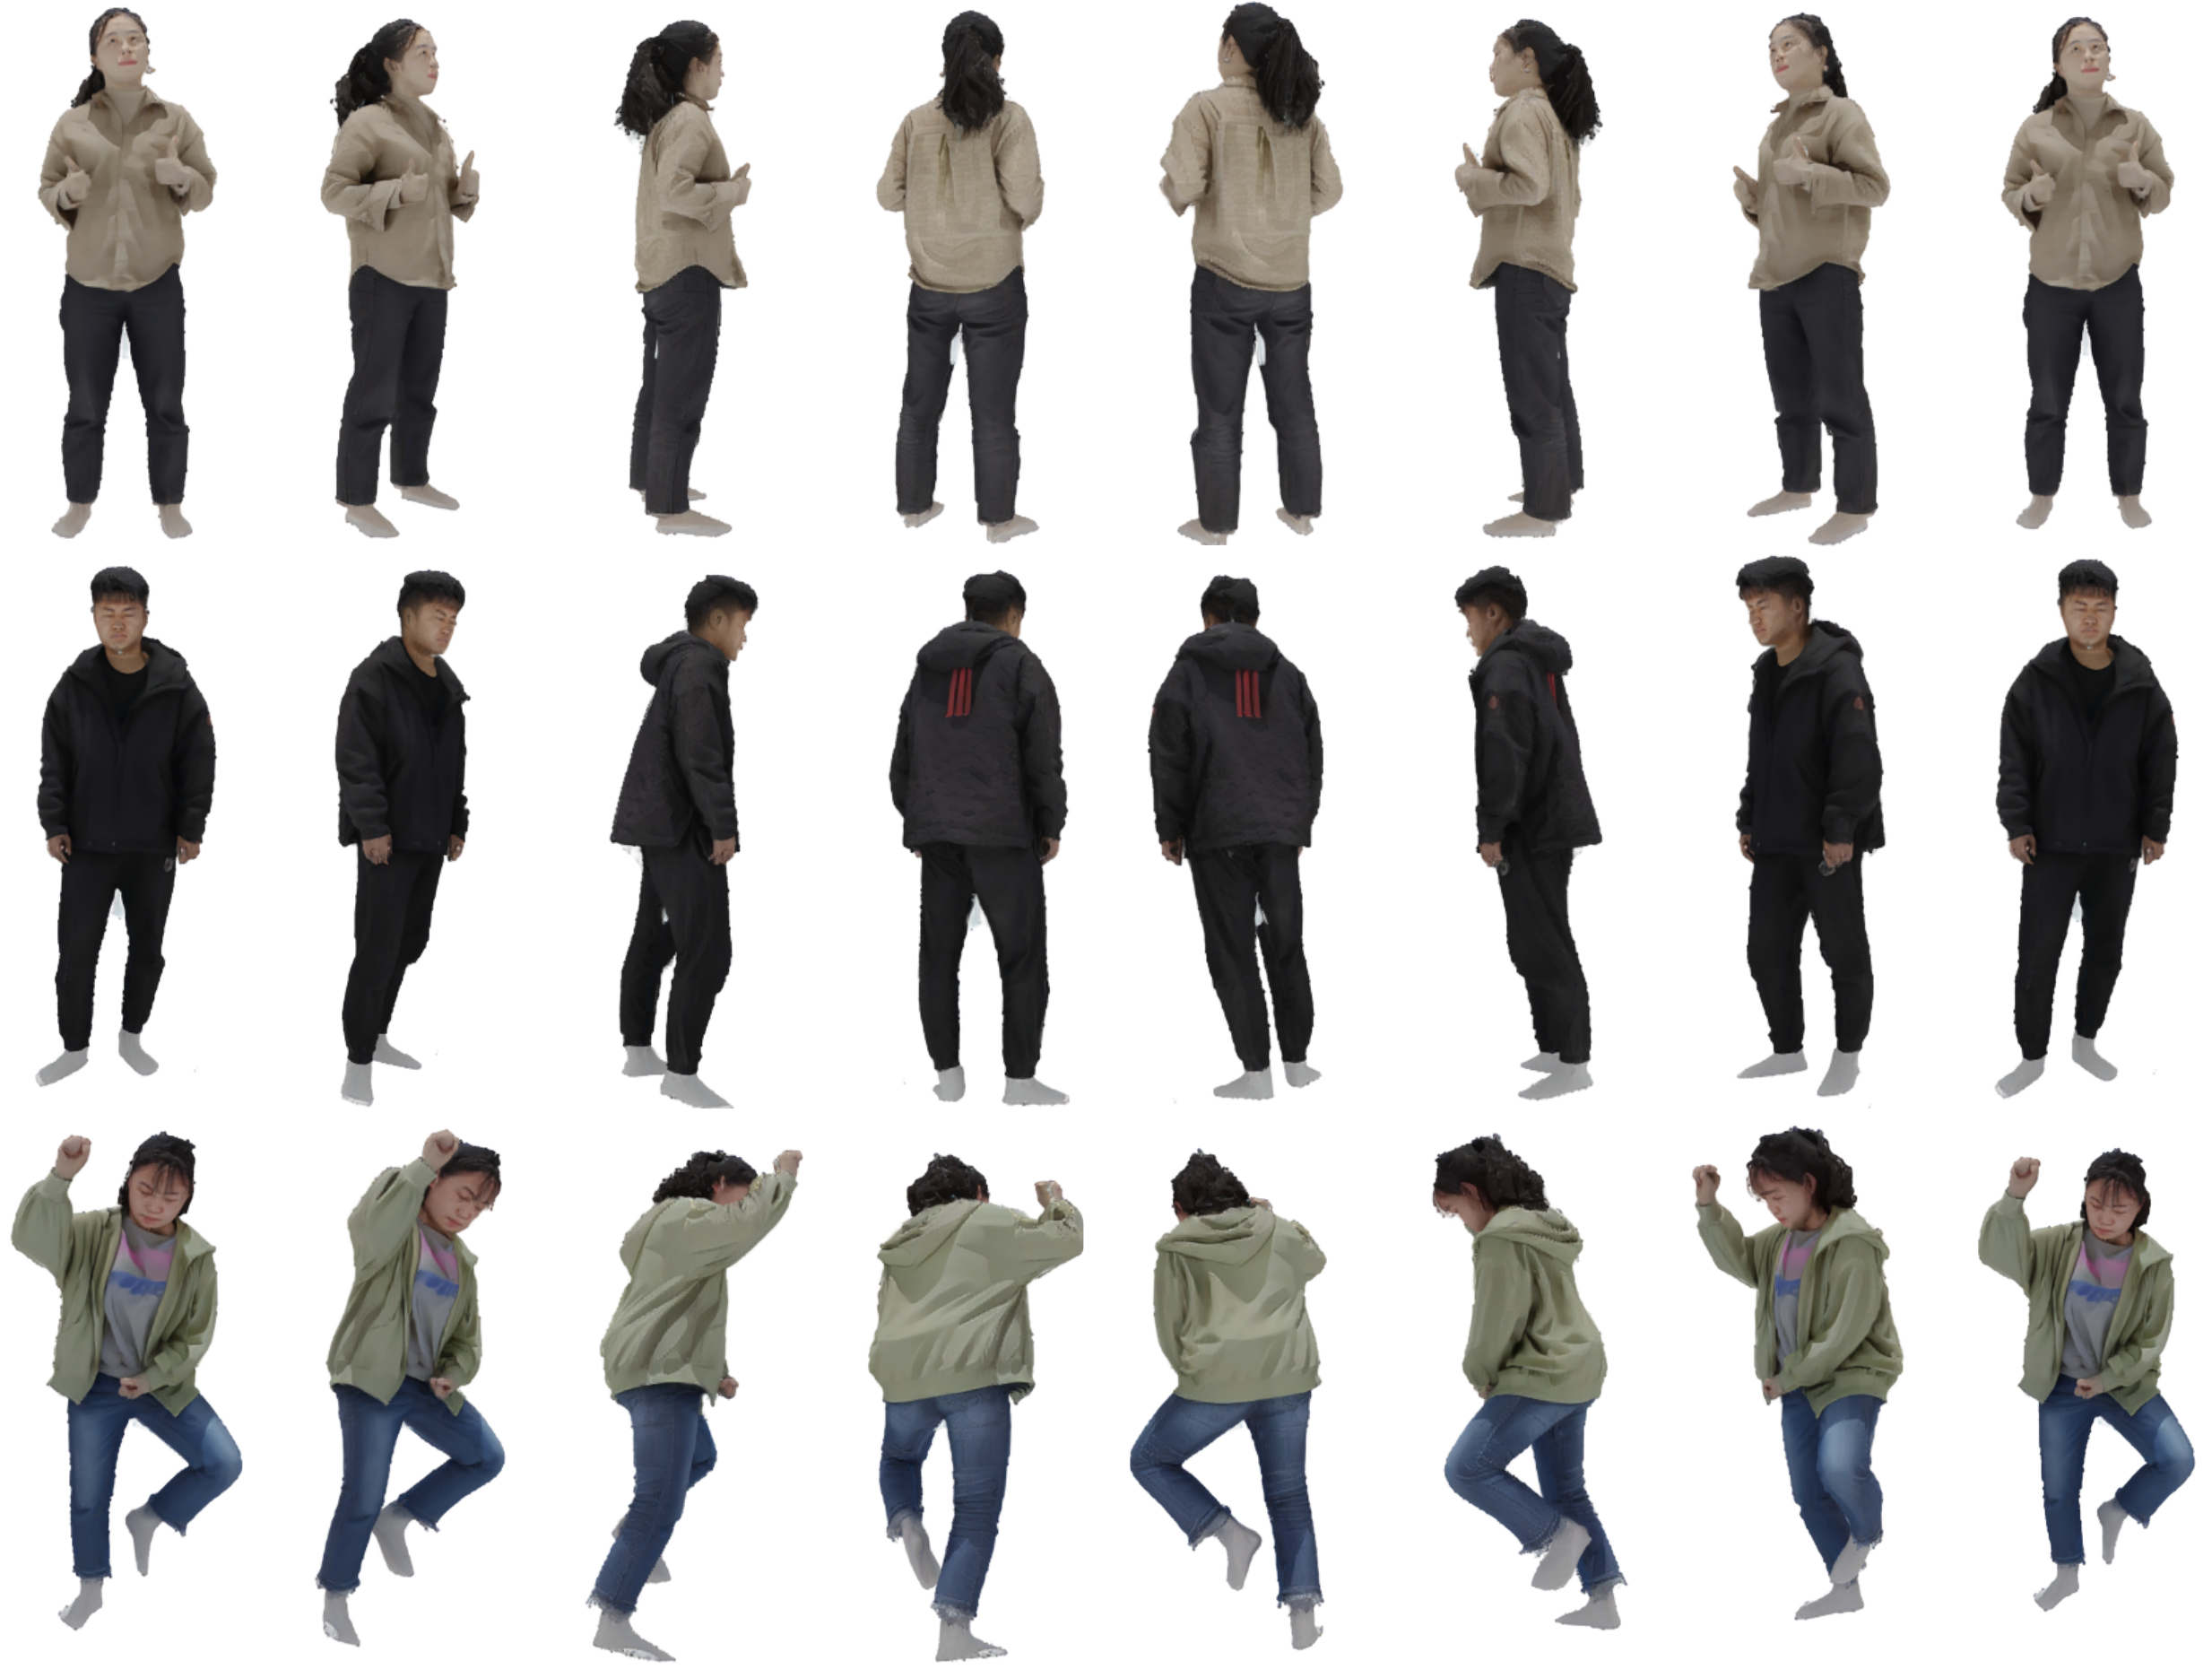}
\caption{Visualization results of applying our model to 3D Gaussian network reconstruction. The input consists of six images captured from different viewpoints.} %Using a finetuned network based on the LGM model \cite{tang2024lgm}, we generate a 3D Gaussian representation. To evaluate the reconstruction, this 3D Gaussian representation is rendered into eight novel views, producing the final results.}
\label{fig:suppl_gs}
\end{figure}

\section{Additional Multi-View Qualitative Results}
\label{sec:supp_mutli_qualitative_res}
Additional results of the THuman2.1 are shown in Figure \ref{fig:suppl_6_views}. Due to limitations in the human data, some viewpoints do not detect faces, so we learn the representation for only three of them. The results include six different viewpoints generated by our model: the first three columns represent outputs that have undergone two stages of representation learning, while the last three columns reflect outputs derived from body representation learning only.

\section{Additional 3D Qualitative Results}
\label{sec:supp_gs_qualitative_res}
In Figure \ref{fig:suppl_gs}, we display the results from 3D gaussian splatting. To be specific, we use the results of our reconstruction as input to a 3D Gaussian network \cite{tang2024lgm}. The number of input images is 6, containing the results of the 3 views obtained after two stages of representation learning and the results obtained after only the body representation learning stage.The result of the visualisation contains 8 views rendered from gaussian splatting. From the results, we can know that our method can be applied to generate 3D Gaussian with consistent viewpoints and high quality results.

\section{Additional Ablation Studies}
\label{sec:supp_abl}
We provide more ablation studies in this section, including the design of the transferred face representation. We directly apply our method to refine the facial images generated from the fine-tuned wonder3d model. In Table \ref{tab:supp_abl_body}, w/o. Body Representation means that results used to calculate quantitative metrics are generated from our method only with transferred face representation.  It can be observed that methods without transferred body representation produces lower human multi-views quality.

\begin{table}
\centering
\resizebox{0.9\linewidth}{!}{
\begin{tabular}{l|ccc}
\toprule
   \textbf{Methods} & PSNR$\uparrow$ & SSIM$\uparrow$ & LPIPS$\downarrow$ \\
\midrule
    Ours (Full) &\textbf{27.130} &\textbf{0.986} &\textbf{0.022}\\
\midrule
    w/o. Body Representation  &25.532  &0.9324 &0.059 \\
\bottomrule
\end{tabular}}
\caption{Ablation study for the transferred face representation learning stage.}
\label{tab:supp_abl_body}
\end{table}

\begin{figure*}
\centering
\includegraphics[width=1\linewidth]{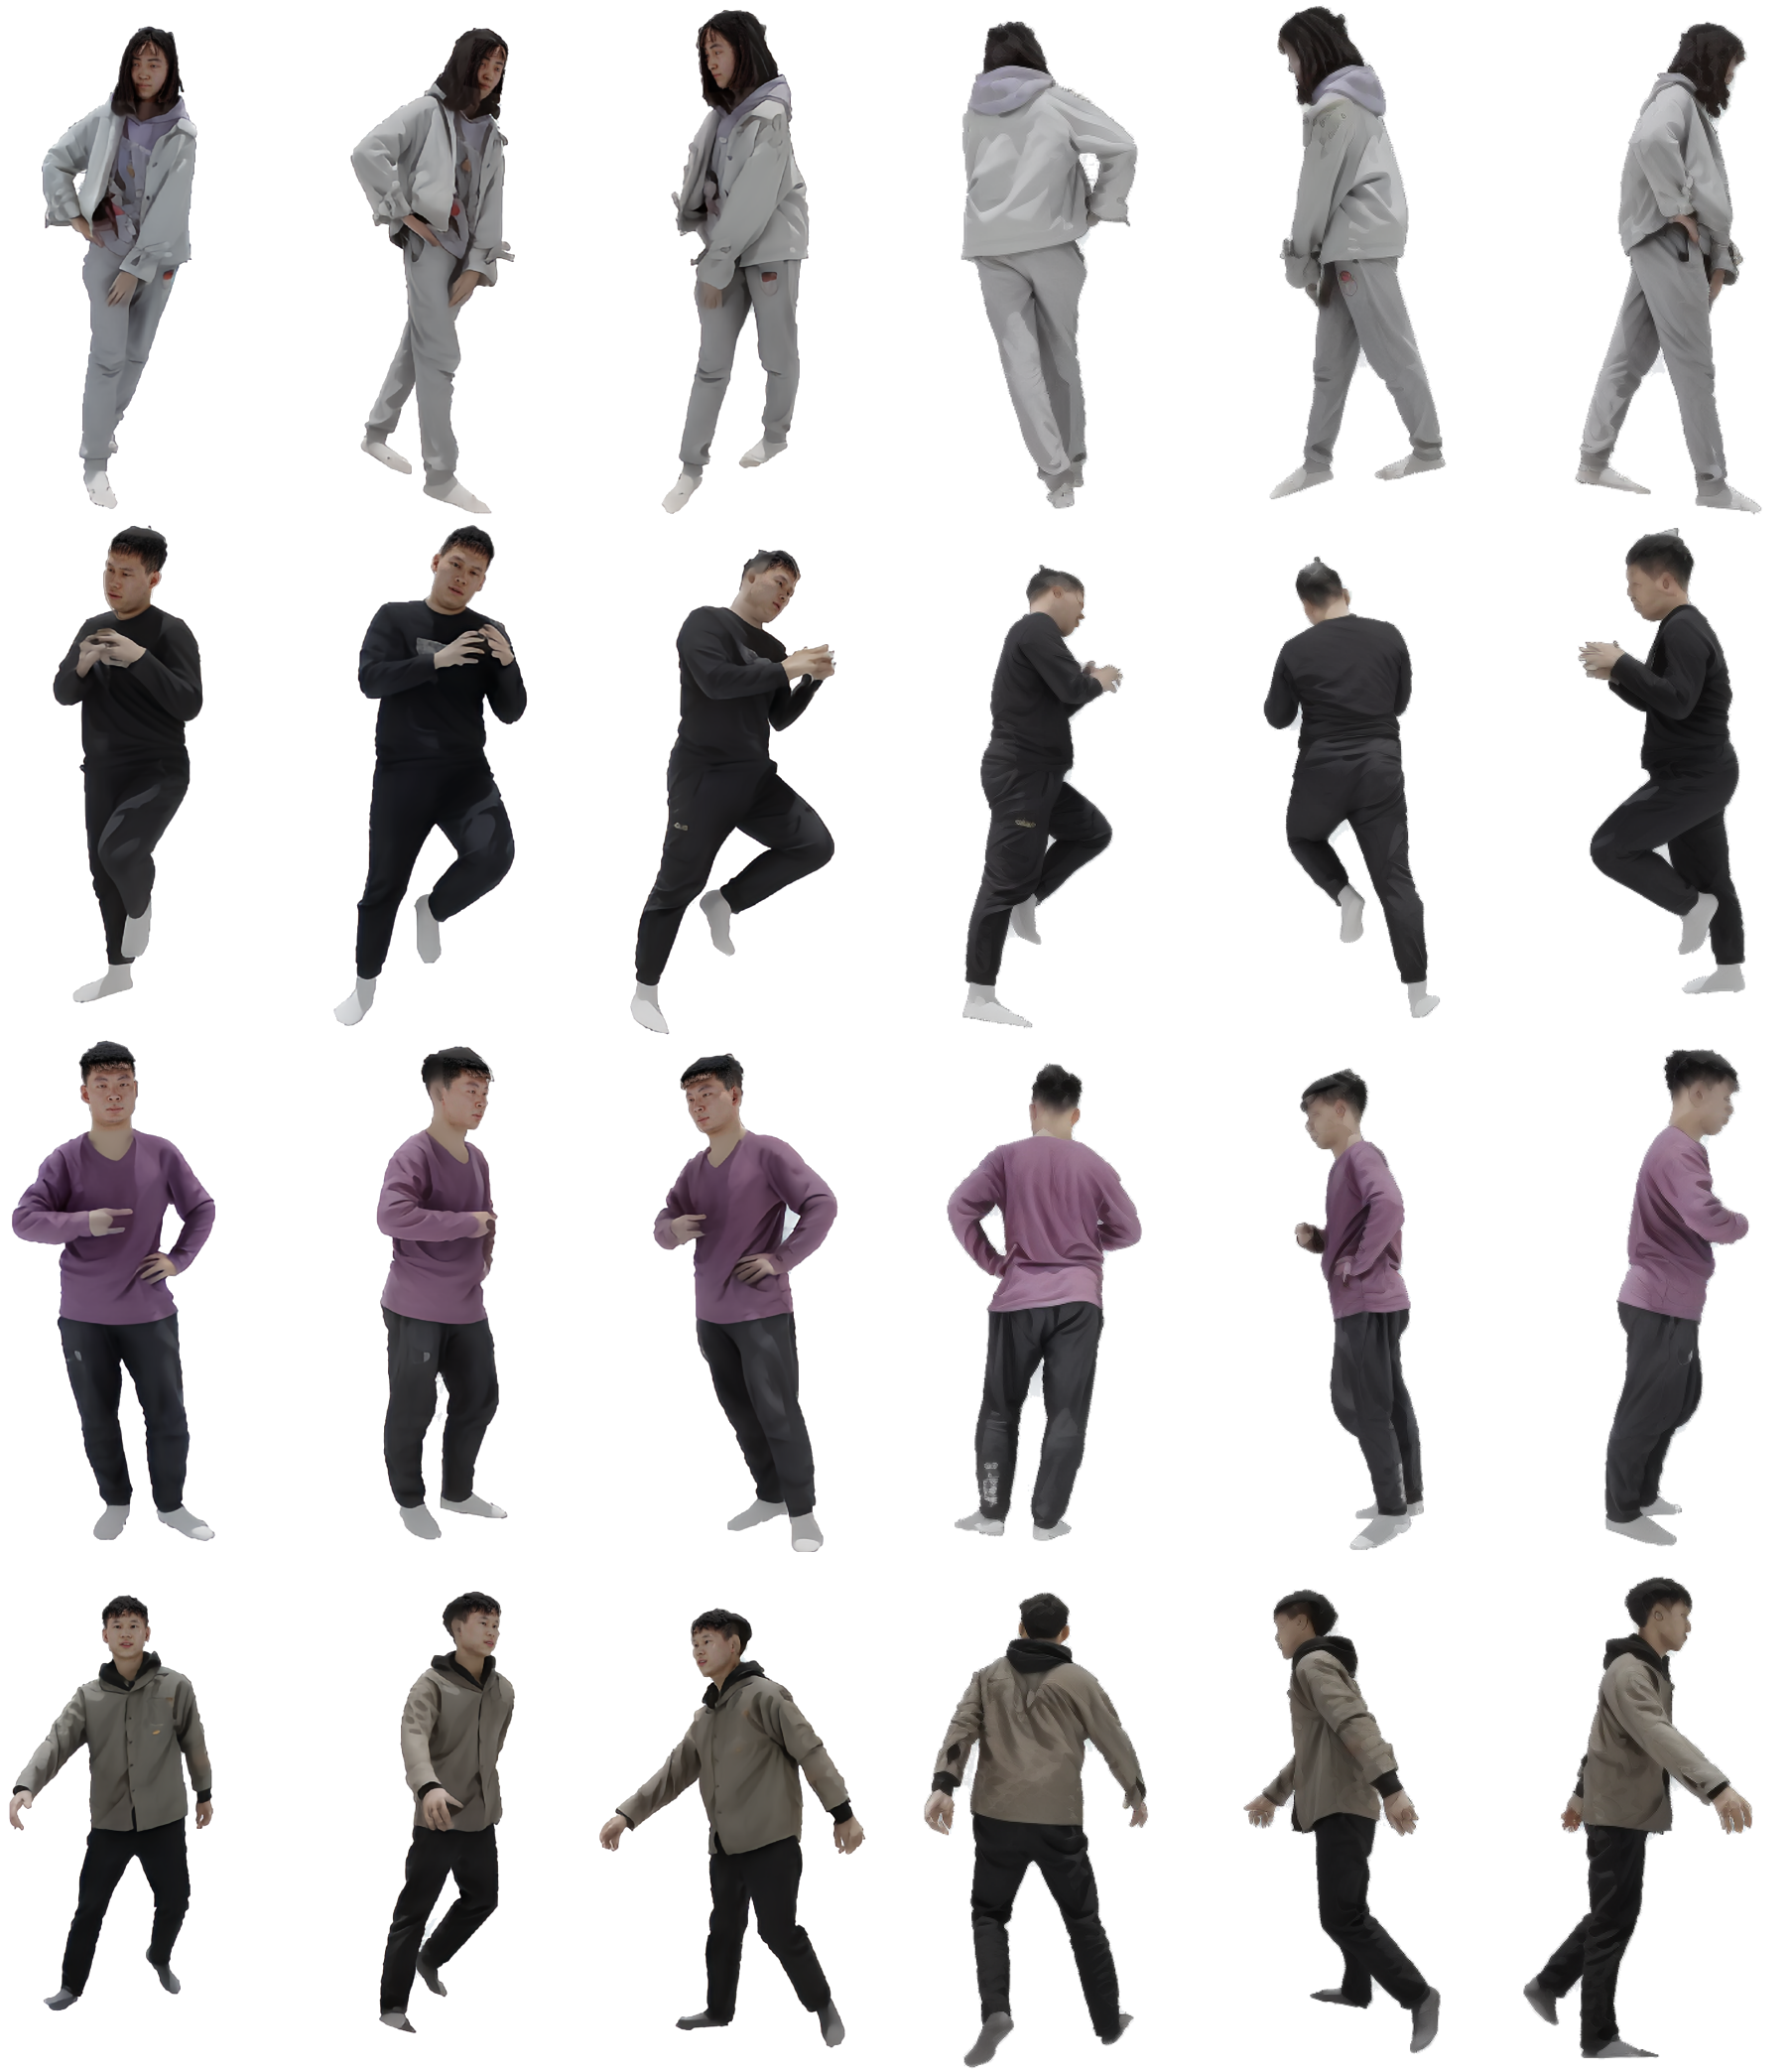}
\caption{Additional qualitative results of our method on THuman2.1.}
\label{fig:suppl_6_views}
\end{figure*}
